# Supplementary material for: In-context Reinforcement Learning with Algorithm Distillation
Source: arXiv:2210.14215 source file (2022-10-25)
Supplement: Supplementary file 1 [file old_appendix.tex]

\begin{comment}

\section{Adversarial Dark Room}
\label{app:ood_9x9}
We extend the adversarial bandit experiments to the Dark Room environment. The environment remains the same (room size of $9 \times 9$, episode length of $20$ and the agent resets at the origin) except that the goal's locations at evaluation time are out of distribution. Training goals have negative abscissa and evaluation goals have positive abscissa. During training, goals are sampled from the evaluation set $10\%$ of the time with a maximum number of different goals in $\{1, 10, 20, 30\}$. At test time, the agent only sees goals with $x>0$. 


\begin{figure}[h]
\centering
\includegraphics[width=\textwidth]{assets/images/ood_9x9.pdf}
\caption{\fullname In-context learning as a function of the number of different goals. The source data for AD comes from learning history from A3C.
We collect a total of $92 400 000$ transitions. The performance improves as more evaluation goals are visited. Even with one evaluation goal seen during training ($10\%$ of the time), the agent shows in-context learning and is able to reach a reward of $0.6$.}
\label{fig:ood_9x9}
\end{figure}

\begin{figure}[h]
\centering
\includegraphics[width=0.9\textwidth]{assets/images/ood_9x9_rl2.pdf}
\caption{$\text{RL}^2$ In-context learning as a function of the number of different goals. We trained on $960 000 000$ transitions. As expected, $\text{RL}^2$ shows slightly better performance than AD when more goals are seen during training. However AD outperforms $\text{RL}^2$ for strongly out-of-distribution goals.}
\label{fig:ood_9x9}
\end{figure}

\begin{figure}[h]
\centering
\includegraphics[width=\textwidth]{assets/images/ood_ablation_1goal.pdf}
\caption{Effect of random sampling and random cropping on AD's performance. Top row: vanilla Dark Room environment. Last row: Dark Room with one evaluation goal seen during training. The best configuration (random sampling, cropping) is consistent in the two cases.}
\label{fig:ood_9x9}
\end{figure}

\begin{figure}
\centering
% \begin{subfigure}{.5\textwidth}
  \centering
  \includegraphics[width=.5\textwidth]{assets/images/attention.pdf}
  \caption{Attention maps from five separate seeds. The left column plots attention for an AD transformer after 200 time-steps (when the context is initially filled). The right column plots attention after 30 episodes.  }
  \label{fig:sub1}
% \end{subfigure}%
% \begin{subfigure}{.5\textwidth}
%   \centering
%   \includegraphics[width=.9\textwidth]{assets/images/attention.png}
%   \caption{A subfigure}
%   \label{fig:sub2}
% \end{subfigure}
% \caption{A figure with two subfigures}
\label{fig:test}
\end{figure}
% \clearpage
% \input{figures/main}
\end{comment}
